# Supplementary material for: Initial Guesses for Multicomponent Mean-Field Methods: Assessment and New Developments
Source: arXiv:2602.11013 ancillary file (2026-02-17)
Supplement: Supplementary file 1 [file supplementary_material.pdf]

# – Supporting Information –

## Initial Guesses for Multicomponent Mean-Field Methods: Assessment and New Developments

Denis G. Artiukhin[1]

Institut für Chemie und Biochemie, Freie Universität Berlin,

Arnimallee 22, 14195 Berlin, Germany

[1]Email: denis.artiukhin@fu-berlin.de

# S1 Additional Theory Aspects

## S1.1 Density Matrix Projections

We start from denoting the original basis set (basis 1) of HO functions with Greek letters $|\alpha\rangle$, and using Roman letters $|i\rangle$ for the final basis set (basis 2) applied in NEO computations. The projector operator onto basis 2 takes the form,

$$\hat{\rho} = \sum_{i,j} |i\rangle \left(\mathbf{S}_{22}\right)^{-1}_{ij} \langle j| \,, \tag{1}$$

where $\mathbf{S}_{22}$ is the overlap matrix in basis 2, i.e., for the set of functions $|i\rangle$. Note that $\hat{\rho} = \hat{I}$ in the same basis set. Let us assume that there exists a function $|A\rangle$, which is represented as a linear combination of basis functions $|\alpha\rangle$,

$$|A\rangle = \sum_{\alpha} A_{\alpha} |\alpha\rangle \,. \tag{2}$$

We can represent this function in the new basis set $|i\rangle$ by projecting it such that,

$$\hat{\rho} |A\rangle = \sum_{i} A_i |i\rangle \,, \tag{3}$$

where new coefficients $A_i$ are given as

$$A_i = \sum_{j,\alpha} \left(\mathbf{S}_{22}\right)^{-1}_{ij} \left(\mathbf{S}_{21}\right)_{j\alpha} A_{\alpha} \tag{4}$$

and $\mathbf{S}_{21}$ contains overlaps of basis functions $|i\rangle$ and $|\alpha\rangle$. Collecting initial $A_{\alpha}$ and final $A_i$ coefficients into the coefficient matrices $\mathbf{C}_1$ and $\mathbf{C}_2$, respectively, the transformation between these can be written in a matrix form,

$$\mathbf{C}_2 = \mathbf{S}_{22}^{-1} \mathbf{S}_{21} \mathbf{C}_1. \tag{5}$$

With this expression, we can now derive the corresponding transformation for density matrices defined in different basis sets. Our first/initial density matrix $\mathbf{P}_1$ is given as

$$\mathbf{P}_1 = \mathbf{C}_1\mathbf{C}_1^{\mathrm{T}}. \tag{6}$$

Note that since a single HO wave function is employed in our approach, the density matrix $\mathbf{P}_1$ becomes a scalar value equal to one. The expression for the second density matrix $\mathbf{P}_2$ reads,

$$\mathbf{P}_2 = \mathbf{C}_2\mathbf{C}_2^{\mathrm{T}} = \mathbf{S}_{22}^{-1}\mathbf{S}_{21}\mathbf{C}_1\mathbf{C}_1^{\mathrm{T}}\mathbf{S}_{21}^{\mathrm{T}}\mathbf{S}_{22}^{-1} = \mathbf{S}_{22}^{-1}\mathbf{S}_{21}\mathbf{P}_1\mathbf{S}_{21}^{\mathrm{T}}\mathbf{S}_{22}^{-1} = \mathbf{U}\mathbf{P}_1\mathbf{U}^{\mathrm{T}}, \tag{7}$$

where the transformation matrix $\mathbf{U}$ is defined by

$$\mathbf{U} = \mathbf{S}_{22}^{-1}\mathbf{S}_{21}. \tag{8}$$

## S1.2 Analytical Expressions for Overlap Integrals

The analytical solution for overlaps from Eq. (16) in the main text can be derived by considering a closely related Gaussian integral [1],

$$Z(\mathbf{A}, \mathbf{b}) = \int_{-\infty}^{+\infty} \exp\left(-\frac{1}{2}\mathbf{Q}^{\mathrm{T}}\mathbf{A}^{-1}\mathbf{Q} + \mathbf{b}^{\mathrm{T}}\mathbf{Q}\right) \mathrm{d}\mathbf{Q} = \frac{(2\pi)^{3/2}}{\sqrt{\det(\mathbf{A}^{-1})}} \exp\left(\frac{1}{2}\mathbf{b}^{\mathrm{T}}\mathbf{A}\mathbf{b}\right), \tag{9}$$

with a linear term $\mathbf{b}^{\mathrm{T}}\mathbf{Q}$ where $\mathbf{b} \in \mathbb{R}^3$ is a vector. Taking partial derivatives of this expression with respect to the components of $\mathbf{b}$ results in,

$$\frac{\partial^l}{\partial b_x^l}\frac{\partial^m}{\partial b_y^m}\frac{\partial^n}{\partial b_z^n} Z(\mathbf{A}, \mathbf{b}) = \int_{-\infty}^{+\infty} Q_x^l Q_y^m Q_z^n \exp\left(-\mathbf{Q}^{\mathrm{T}}\mathbf{A}^{-1}\mathbf{Q} + \mathbf{b}^{\mathrm{T}}\mathbf{Q}\right) \mathrm{d}\mathbf{Q}. \tag{10}$$

Therefore, the integral $\langle\psi|\chi_{lmn}\rangle$ can be evaluated by taking partial derivatives of the analytical solution from Eq. (9) and considering the case of $\mathbf{b} = \mathbf{0}$, i.e.,

$$\langle\psi|\chi_{lmn}\rangle = N_\psi N_{lmn} \frac{(2\pi)^{3/2}}{\sqrt{\det(\mathbf{A}^{-1})}} \left[ \frac{\partial^l}{\partial b_x^l} \frac{\partial^m}{\partial b_y^m} \frac{\partial^n}{\partial b_z^n} \exp\left(\frac{1}{2}\mathbf{b}^\mathrm{T}\mathbf{A}\mathbf{b}\right)\right]\Bigg|_{\mathbf{b}=\mathbf{0}} . \tag{11}$$

Here, we provide an explicit derivation of the overlap integrals given in Eq. (11). For this, we evaluate the normalized cumulants of the form

$$\left[ \frac{\partial^{n_x}}{\partial b_x^{n_x}} \frac{\partial^{n_y}}{\partial b_y^{n_y}} \frac{\partial^{n_z}}{\partial b_z^{n_z}} \exp\left(\frac{1}{2}\mathbf{b}^\mathrm{T}\mathbf{A}\mathbf{b}\right)\right]\Bigg|_{\mathbf{b}=\mathbf{0}} . \tag{12}$$

The expression under the exponent, which we denote $w$, can be written as

$$w(\mathbf{b}) = \frac{1}{2}\mathbf{b}^\mathrm{T}\mathbf{A}\mathbf{b} = \frac{1}{2}\sum_{i=1}^{3}\sum_{j=1}^{3} A_{ij} b_i b_j , \tag{13}$$

where $x, y, z$ are denoted with indices $i, j \in \{1, 2, 3\}$. The overlap with the $s$-functions ($n_x + n_y + n_z = 0$) is given as

$$\left[\exp\left(\frac{1}{2}w(\mathbf{b})\right)\right]\Bigg|_{\mathbf{b}=\mathbf{0}} = 1 . \tag{14}$$

For the $p$-functions ($n_x + n_y + n_z = 1$), we obtain

$$\left[\frac{\partial}{\partial b_k}\exp\left(w(\mathbf{b})\right)\right]\Bigg|_{\mathbf{b}=\mathbf{0}} = \left[(\mathbf{A}_k \cdot \mathbf{b})\exp\left(w(\mathbf{b})\right)\right]\big|_{\mathbf{b}=\mathbf{0}} = 0 , \tag{15}$$

where

$$\mathbf{A}_k \cdot \mathbf{b} = \sum_{i=1}^{3} A_{ik} b_i . \tag{16}$$

For $d$-functions ($n_x + n_y + n_z = 2$), the expression reads

$$\left[\frac{\partial}{\partial b_k}\frac{\partial}{\partial b_l}\exp\left(w(\mathbf{b})\right)\right]\Bigg|_{\mathbf{b}=\mathbf{0}} = \left[\left((\mathbf{A}_k \cdot \mathbf{b})(\mathbf{A}_l \cdot \mathbf{b}) + A_{kl}\right)\exp\left(w(\mathbf{b})\right)\right]\big|_{\mathbf{b}=\mathbf{0}} = A_{kl} . \tag{17}$$

For $f$-functions ($n_x + n_y + n_z = 3$), we obtain

$$\left[\frac{\partial}{\partial b_k}\frac{\partial}{\partial b_l}\frac{\partial}{\partial b_m}\exp\left(w(\mathbf{b})\right)\right]\Bigg|_{\mathbf{b}=\mathbf{0}} = \left[f_3 \exp\left(w(\mathbf{b})\right)\right]\big|_{\mathbf{b}=\mathbf{0}} = 0 \ , \tag{18}$$

where $f_3$ is a polynomial of third order in $\mathbf{b}$,

$$f_3 = (\mathbf{A}_k \cdot \mathbf{b})(\mathbf{A}_l \cdot \mathbf{b})(\mathbf{A}_m \cdot \mathbf{b}) + A_{kl}(\mathbf{A}_m \cdot \mathbf{b}) + A_{lm}(\mathbf{A}_k \cdot \mathbf{b}) + A_{mk}(\mathbf{A}_l \cdot \mathbf{b}). \tag{19}$$

Finally, for $g$-functions ($n_x + n_y + n_z = 4$), we have

$$\left[\frac{\partial^2}{\partial b_k^2}\frac{\partial}{\partial b_l}\frac{\partial}{\partial b_m}\exp\left(w(\mathbf{b})\right)\right]\Bigg|_{\mathbf{b}=\mathbf{0}} = \left[f_4 \exp\left(w(\mathbf{b})\right)\right]\big|_{\mathbf{b}=\mathbf{0}} = A_{kl}A_{mk} + A_{km}A_{lk} + A_{lm}A_{kk} \ , \tag{20}$$

where

$$\begin{aligned} f_4 = {} & (\mathbf{A}_k \cdot \mathbf{b})^2(\mathbf{A}_l \cdot \mathbf{b})(\mathbf{A}_m \cdot \mathbf{b}) \\ & + (\mathbf{A}_k \cdot \mathbf{b})(A_{kl}(\mathbf{A}_m \cdot \mathbf{b}) + A_{lm}(\mathbf{A}_k \cdot \mathbf{b}) + A_{mk}(\mathbf{A}_l \cdot \mathbf{b})) \\ & + A_{kl}A_{mk} + A_{km}A_{lk} + A_{lm}A_{kk} \ . \end{aligned} \tag{21}$$

The integral evaluation for $h$-functions ($n_x + n_y + n_z = 5$) leads to zero, due to the aforementioned symmetry.

Table S1: Analytical expressions for $M_{lmn}$ values. See the main text for more details.

| $(lmn)$ | $M_{lmn}$ |
|---|---|
| s-functions | |
| (000) | 1 |
| d-functions | |
| (200) | $A_{11}$ |
| (020) | $A_{22}$ |
| (002) | $A_{33}$ |
| (110) | $A_{12}$ |
| (101) | $A_{13}$ |
| (011) | $A_{23}$ |
| g-functions | |
| (400) | $3A_{11}^2$ |
| (040) | $3A_{22}^2$ |
| (004) | $3A_{33}^2$ |
| (310) | $3A_{11}A_{12}$ |
| (301) | $3A_{11}A_{13}$ |
| (031) | $3A_{22}A_{23}$ |
| (130) | $3A_{22}A_{21}$ |
| (103) | $3A_{33}A_{31}$ |
| (013) | $3A_{33}A_{32}$ |
| (220) | $2A_{12}^2 + A_{11}A_{22}$ |
| (202) | $2A_{13}^2 + A_{11}A_{33}$ |
| (022) | $2A_{23}^2 + A_{22}A_{33}$ |
| (211) | $2A_{12}A_{31} + A_{23}A_{11}$ |
| (121) | $2A_{21}A_{32} + A_{13}A_{22}$ |
| (112) | $2A_{31}A_{23} + A_{12}A_{33}$ |

## S2 Comparison of QChem and Serenity

To verify the correctness of the NEO-HF [2] and NEO-DFT [3–7] program implementations in Serenity [8–10], total NEO-SCF energies were compared against those generated with the Q-Chem 6.2 software [11]. To that end, computational settings in both packages were chosen such that protocols are as similar as possible and deviations in the energies are minimal. In case of Serenity, the computational protocol for NEO-DFT and NEO-HF is same as provided in the main text with a restriction of testing only one spherical protonic PB4-D basis set [12]. Additionally a computational scheme, where NEO-DFT is applied without an electron–proton correlation functional was applied. In case of Q-Chem, apart from same major computational settings being employed (i.e., functionals and basis sets), the following thresholds were set. The cutoffs for overlap matrix elements and two-electron integrals being ignored were both set to $1.0\times10^{-14}$. SCF convergence thresholds for electronic and nuclear wave function errors were set to $1.0\times10^{-8}$. The acceptable energy difference between consecutive NEO-SCF iterations was specified to be equal to $1.0\times10^{-8}$ a.u. Stepwise NEO-SCF convergence protocol was used in all cases. Default integration grids were employed in Q-Chem. Results of these assessment are summarized in the tables below.

Table S2: Comparison of NEO-HF energies obtained with the Serenity and Q-Chem program packages. Deviating digits and protons, which were treated as quantum, are given in bold fonts. All values are provided in a.u.

| Molecule | Serenity | Q-Chem | $\lvert\Delta E\rvert$ |
|---|---|---|---|
| F**H**F$^-$ | −199.546017693**7** | -199.546017693**2** | $5.00\times10^{-10}$ |
| **H**CN | −92.8689951**138** | −92.8689951**315** | $1.77\times10^{-8}$ |
| $\mathbf{H}_2$O | −76.0190045**6441** | −76.0190045**5515** | $9.26\times10^{-8}$ |
| C$\mathbf{H}_2$O | −113.8283701**375** | −113.8283701**485** | $1.10\times10^{-8}$ |
| $C_2\mathbf{H}_4$ | −77.8934812**969** | −77.8934812**860** | $1.09\times10^{-8}$ |

Table S3: Comparison of NEO-DFT energies obtained with the Serenity and Q-Chem program packages without using an electron–proton correlation functional. Deviating digits and protons, which were treated as quantum, are given in bold fonts. All values are provided in a.u.

| Molecule | Serenity | Q-Chem | $\lvert\Delta E\rvert$ |
|---|---|---|---|
| F**H**F$^{-}$ | −200.2304**165350** | −200.2304**083331** | $8.20\times10^{-6}$ |
| **H**CN | −93.30395**32461** | −93.30395**61430** | $2.90\times10^{-6}$ |
| $\mathbf{H}_2$O | −76.33892**98850** | −76.33892**02232** | $9.66\times10^{-6}$ |
| C$\mathbf{H}_2$O | −114.33142**54958** | −114.33142**31463** | $2.35\times10^{-6}$ |
| $C_2\mathbf{H}_4$ | −78.3290**873888** | −78.3290**559438** | $3.14\times10^{-5}$ |

Table S4: Comparison of NEO-DFT energies obtained with the Serenity and Q-Chem program packages using the EPC17-2 electron–proton correlation functional. Deviating digits and protons, which were treated as quantum, are given in bold fonts. All values are provided in a.u.

| Molecule | Serenity | Q-Chem | $\lvert\Delta E\rvert$ |
|---|---|---|---|
| F**H**F$^{-}$ | −200.258**5051643** | −200.258**4970607** | $8.10\times10^{-6}$ |
| **H**CN | −93.33137**97562** | −93.33137**47039** | $5.05\times10^{-6}$ |
| $\mathbf{H}_2$O | −76.36699**75363** | −76.36699**08408** | $6.70\times10^{-6}$ |
| C$\mathbf{H}_2$O | −114.3854794**152** | −114.3854798**320** | $4.17\times10^{-7}$ |
| $C_2\mathbf{H}_4$ | −78.4375**803617** | −78.4375**527529** | $2.76\times10^{-5}$ |

# S3 $f$-Rank Scores

Table S5: $f$-rank scores computed with NEO-HF using Cartesian protonic basis sets. Bold fonts denote protons, which were treated as quantum particles. Omitted values correspond to computations, which did not converge or converged to wrong minima.

| Molecule | PB4-D | | | | PB4-F1 | | | | PB4-F2 | | | |
|---|---|---|---|---|---|---|---|---|---|---|---|---|
| | HOa | HOi | 1s | core | HOa | HOi | 1s | core | HOa | HOi | 1s | core |
| F**H**F$^-$ | 0.54 | 0.66 | 0.98 | 1.00 | 0.54 | 0.66 | 0.98 | 1.00 | 0.54 | 0.66 | 0.98 | 1.00 |
| HO**H**$\cdots$FH | 0.42 | 0.94 | 0.95 | 0.98 | 0.43 | 0.94 | 0.95 | 0.98 | 0.43 | 0.94 | 0.94 | 0.98 |
| HO**H**$\cdots$ClH | 0.26 | 0.89 | 0.96 | 0.98 | 0.26 | 0.89 | 0.96 | 0.98 | 0.26 | 0.89 | 0.96 | 0.98 |
| $H_2O\cdots$**H**OH | 0.44 | 0.93 | 0.95 | 0.98 | 0.44 | 0.93 | 0.95 | 0.98 | 0.44 | 0.93 | 0.95 | 0.98 |
| $CH_3OH\cdots$**H**OH | 0.45 | 0.93 | 0.96 | 0.98 | 0.45 | 0.93 | 0.96 | 0.98 | 0.45 | 0.93 | 0.95 | 0.98 |
| H**H**NO | 0.57 | 0.88 | 0.96 | 0.98 | 0.57 | 0.88 | 0.96 | 0.98 | 0.57 | 0.88 | 0.96 | 0.98 |
| HO**H** | 0.59 | 0.93 | 0.96 | 0.98 | 0.59 | 0.93 | 0.96 | 0.98 | 0.59 | 0.93 | 0.96 | 0.98 |
| HS**H** | 0.48 | 0.85 | 0.97 | 0.98 | 0.48 | 0.85 | 0.97 | 0.98 | 0.48 | 0.85 | 0.97 | 0.98 |
| **H**CN | 0.42 | 0.89 | 0.96 | 0.98 | 0.42 | 0.89 | 0.96 | 0.98 | 0.42 | 0.89 | 0.96 | 0.98 |
| **H**FCO | 0.52 | 0.85 | 0.96 | 0.98 | 0.52 | 0.85 | 0.96 | 0.98 | 0.52 | 0.85 | 0.96 | 0.98 |
| **H**NO | 0.64 | 0.86 | 0.96 | 0.98 | 0.64 | 0.86 | 0.96 | 0.98 | 0.64 | 0.86 | 0.96 | 0.98 |
| **H**OCl | 0.63 | 0.93 | 0.96 | 0.98 | 0.63 | 0.93 | 0.96 | 0.98 | 0.63 | 0.93 | 0.96 | 0.98 |
| **H**OF | 0.67 | 0.93 | 0.96 | 0.98 | 0.67 | 0.93 | 0.96 | 0.98 | 0.67 | 0.93 | 0.95 | 0.98 |
| **H**ONO | 0.47 | 0.93 | 0.96 | 0.98 | 0.47 | 0.93 | 0.96 | 0.98 | 0.47 | 0.93 | 0.95 | 0.98 |
| $C\mathbf{H}_2O$ | 0.49 | 0.84 | 0.97 | 0.87 | 0.49 | 0.84 | 0.97 | 0.87 | 0.49 | 0.84 | 0.97 | 0.86 |
| $C\mathbf{H}_3F$ | 0.57 | 0.85 | 0.97 | 0.72 | 0.57 | 0.85 | 0.97 | 0.72 | 0.57 | 0.85 | 0.97 | 0.72 |
| $C_2\mathbf{H}_4$ | 0.51 | 0.86 | 0.97 | 0.80 | 0.51 | 0.86 | 0.97 | 0.80 | 0.51 | 0.86 | 0.97 | 0.80 |
| $\mathbf{H}_2O\cdots\mathbf{H}F$ | 0.34 | 0.94 | 0.95 | 0.83 | 0.34 | 0.93 | 0.95 | 0.82 | 0.34 | 0.93 | 0.95 | 0.82 |
| $\mathbf{H}_2O\cdots\mathbf{H}Cl$ | 0.48 | – | – | 0.84 | 0.49 | 0.92 | 0.96 | 0.84 | 0.49 | 0.92 | 0.96 | 0.83 |
| $\mathbf{H}_2O\cdots\mathbf{H}_2O$ | 0.30 | 0.93 | 0.96 | 0.78 | – | – | – | 0.77 | – | – | – | 0.77 |

Table S6: $f$-rank scores computed with NEO-HF using spherical protonic basis sets. Bold fonts denote protons, which were treated as quantum particles. Omitted values correspond to computations, which did not converge or converged to wrong minima.

| Molecule | PB4-D | | | PB4-F1 | | | PB4-F2 | | |
|---|---|---|---|---|---|---|---|---|---|
| | HOi | 1s | core | HOi | 1s | core | HOi | 1s | core |
| F**H**F$^-$ | 0.66 | 0.98 | 1.00 | 0.66 | 0.98 | 1.00 | 0.66 | 0.98 | 1.00 |
| HO**H**$\cdots$FH | 0.94 | 0.95 | 0.98 | 0.94 | 0.95 | 0.98 | 0.94 | 0.95 | 0.98 |
| HO**H**$\cdots$ClH | 0.89 | 0.96 | 0.98 | 0.89 | 0.96 | 0.98 | 0.88 | 0.96 | 0.98 |
| $H_2O\cdots$**H**OH | 0.93 | 0.96 | 0.98 | 0.93 | 0.96 | 0.98 | 0.93 | 0.96 | 0.98 |
| $CH_3OH\cdots$**H**OH | 0.93 | 0.96 | 0.98 | 0.93 | 0.96 | 0.98 | 0.93 | 0.96 | 0.98 |
| H**H**NO | 0.88 | 0.96 | 0.98 | 0.88 | 0.96 | 0.98 | 0.88 | 0.96 | 0.98 |
| HO**H** | 0.93 | 0.96 | 0.99 | 0.93 | 0.96 | 0.99 | 0.93 | 0.96 | 0.99 |
| HS**H** | 0.85 | 0.97 | 0.99 | 0.85 | 0.97 | 0.99 | 0.85 | 0.97 | 0.99 |
| **H**CN | 0.89 | 0.97 | 0.98 | 0.89 | 0.97 | 0.98 | 0.89 | 0.97 | 0.98 |
| **H**FCO | 0.86 | 0.97 | 0.98 | 0.85 | 0.97 | 0.98 | 0.85 | 0.97 | 0.98 |
| **H**NO | 0.86 | 0.96 | 0.98 | 0.86 | 0.96 | 0.98 | 0.86 | 0.96 | 0.98 |
| **H**OCl | 0.93 | 0.96 | 0.99 | 0.93 | 0.96 | 0.99 | 0.93 | 0.96 | 0.98 |
| **H**OF | 0.93 | 0.96 | 0.98 | 0.93 | 0.96 | 0.98 | 0.93 | 0.96 | 0.98 |
| **H**ONO | 0.93 | 0.96 | 0.99 | 0.93 | 0.96 | 0.98 | 0.93 | 0.96 | 0.98 |
| C$\mathbf{H}_2$O | 0.84 | 0.97 | 0.87 | 0.84 | 0.97 | 0.87 | 0.84 | 0.97 | 0.87 |
| C$\mathbf{H}_3$F | 0.85 | 0.97 | 0.73 | 0.85 | 0.97 | 0.73 | 0.85 | 0.97 | 0.73 |
| $C_2\mathbf{H}_4$ | 0.86 | 0.97 | 0.80 | 0.86 | 0.97 | 0.80 | 0.86 | 0.97 | 0.80 |
| $\mathbf{H}_2O\cdots$**H**F | – | – | 0.83 | 0.94 | 0.96 | 0.83 | 0.93 | 0.96 | 0.82 |
| $\mathbf{H}_2O\cdots$**H**Cl | – | – | 0.85 | – | – | 0.84 | – | – | 0.84 |
| $\mathbf{H}_2O\cdots\mathbf{H}_2O$ | 0.93 | 0.96 | 0.78 | 0.93 | 0.96 | 0.78 | 0.93 | 0.96 | 0.77 |

Table S7: $f$-rank scores computed with NEO-HF using spherical protonic basis sets. Bold fonts denote protons, which were treated as quantum particles. Omitted values correspond to computations, which did not converge or converged to wrong minima.

| Molecule | PB5-D | | | PB5-F | | | PB5-G | | |
|---|---|---|---|---|---|---|---|---|---|
| | HOi | 1s | core | HOi | 1s | core | HOi | 1s | core |
| F**H**F$^-$ | 0.66 | 0.98 | 1.00 | 0.66 | 0.98 | 1.00 | 0.66 | 0.98 | 1.00 |
| HO**H**$\cdots$FH | 0.94 | 0.95 | 0.98 | 0.94 | 0.95 | 0.98 | 0.94 | 0.95 | 0.98 |
| HO**H**$\cdots$ClH | 0.89 | 0.96 | 0.98 | 0.88 | 0.96 | 0.98 | 0.88 | 0.96 | 0.98 |
| $H_2O\cdots$**H**OH | 0.93 | 0.96 | 0.98 | 0.93 | 0.96 | 0.98 | 0.93 | 0.96 | 0.98 |
| $CH_3OH\cdots$**H**OH | 0.93 | 0.96 | 0.98 | 0.93 | 0.96 | 0.98 | 0.93 | 0.96 | 0.98 |
| H**H**NO | 0.88 | 0.96 | 0.98 | 0.88 | 0.96 | 0.98 | 0.88 | 0.96 | 0.98 |
| HO**H** | 0.93 | 0.96 | 0.99 | 0.93 | 0.96 | 0.99 | 0.93 | 0.96 | 0.99 |
| HS**H** | 0.85 | 0.97 | 0.99 | 0.85 | 0.97 | 0.99 | 0.85 | 0.97 | 0.99 |
| **H**CN | 0.89 | 0.97 | 0.99 | 0.89 | 0.97 | 0.98 | 0.89 | 0.97 | 0.98 |
| **H**FCO | 0.85 | 0.97 | 0.98 | 0.85 | 0.97 | 0.98 | 0.85 | 0.97 | 0.98 |
| **H**NO | 0.86 | 0.96 | 0.98 | 0.86 | 0.96 | 0.98 | 0.86 | 0.96 | 0.98 |
| **H**OCl | 0.93 | 0.96 | 0.99 | – | – | 0.98 | – | – | 0.98 |
| **H**OF | 0.93 | 0.96 | 0.99 | 0.93 | 0.96 | 0.98 | 0.93 | 0.96 | 0.98 |
| **H**ONO | 0.93 | 0.96 | 0.99 | 0.93 | 0.96 | 0.98 | 0.93 | – | 0.98 |
| C$\mathbf{H_2}$O | 0.84 | 0.97 | 0.87 | 0.84 | 0.97 | 0.87 | 0.84 | 0.97 | 0.87 |
| C$\mathbf{H_3}$F | 0.85 | 0.97 | 0.73 | 0.85 | 0.97 | 0.72 | 0.85 | 0.97 | 0.72 |
| $C_2\mathbf{H_4}$ | 0.86 | 0.97 | 0.80 | 0.86 | 0.97 | 0.80 | 0.86 | 0.97 | 0.80 |
| $\mathbf{H_2}O\cdots$**H**F | 0.94 | 0.96 | 0.83 | 0.93 | 0.96 | 0.82 | 0.93 | 0.96 | 0.82 |
| $\mathbf{H_2}O\cdots$**H**Cl | 0.92 | 0.96 | 0.85 | 0.92 | 0.96 | 0.84 | 0.92 | 0.96 | 0.84 |
| $\mathbf{H_2}O\cdots\mathbf{H_2}O$ | – | 0.96 | 0.78 | 0.93 | – | 0.77 | – | – | 0.77 |

Table S8: $f$-rank scores computed with NEO-DFT using Cartesian protonic basis sets. Bold fonts denote protons, which were treated as quantum particles. Omitted values correspond to computations, which did not converge or converged to wrong minima.

| Molecule | PB4-D | | | | PB4-F1 | | | | PB4-F2 | | | |
|---|---|---|---|---|---|---|---|---|---|---|---|---|
| | HOa | HOi | 1s | core | HOa | HOi | 1s | core | HOa | HOi | 1s | core |
| $F\mathbf{H}F^-$ | 0.92 | 0.94 | 0.69 | 0.74 | 0.92 | 0.94 | 0.69 | 0.74 | 0.92 | 0.94 | 0.69 | 0.74 |
| $H_2O\cdots\mathbf{H}F$ | 0.78 | 0.90 | 0.71 | 0.73 | 0.78 | 0.90 | 0.71 | 0.72 | 0.78 | 0.90 | 0.71 | 0.72 |
| $H_2O\cdots\mathbf{H}Cl$ | 0.66 | 0.97 | 0.73 | 0.75 | 0.66 | 0.97 | 0.72 | 0.74 | 0.66 | 0.97 | 0.72 | 0.74 |
| $H_2O\cdots\mathbf{H}OH$ | 0.78 | 0.91 | 0.75 | 0.74 | 0.78 | 0.91 | 0.74 | 0.74 | 0.78 | 0.91 | 0.74 | 0.73 |
| $CH_3OH\cdots\mathbf{H}OH$ | 0.79 | 0.91 | 0.74 | 0.74 | 0.79 | 0.91 | 0.74 | 0.73 | 0.79 | 0.91 | 0.74 | 0.73 |
| $H\mathbf{H}NO$ | 0.82 | 0.96 | 0.78 | 0.76 | 0.82 | 0.95 | 0.78 | 0.75 | 0.82 | 0.95 | 0.77 | 0.75 |
| $HO\mathbf{H}$ | 0.88 | 0.90 | 0.76 | 0.74 | 0.88 | 0.90 | 0.76 | 0.74 | 0.88 | 0.90 | 0.75 | 0.74 |
| $HS\mathbf{H}$ | 0.30 | 0.98 | 0.77 | 0.76 | 0.30 | 0.98 | 0.77 | 0.76 | 0.30 | 0.97 | 0.77 | 0.76 |
| $\mathbf{H}CN$ | 0.66 | 0.94 | 0.77 | 0.75 | 0.66 | 0.94 | 0.77 | 0.75 | 0.66 | 0.94 | 0.77 | 0.75 |
| $\mathbf{H}FCO$ | 0.79 | 0.96 | 0.80 | 0.77 | 0.79 | 0.96 | 0.79 | 0.76 | 0.79 | 0.96 | 0.79 | 0.76 |
| $\mathbf{H}NO$ | 0.91 | 0.97 | 0.79 | 0.76 | 0.91 | 0.97 | 0.79 | 0.76 | 0.91 | 0.96 | 0.79 | 0.76 |
| $\mathbf{H}OCl$ | 0.90 | 0.91 | 0.76 | 0.74 | 0.89 | 0.91 | 0.76 | 0.74 | 0.89 | 0.90 | 0.75 | 0.74 |
| $\mathbf{H}OF$ | 0.91 | 0.91 | 0.76 | 0.75 | 0.91 | 0.91 | 0.76 | 0.74 | 0.91 | 0.91 | 0.75 | 0.74 |
| $\mathbf{H}ONO$ | 0.75 | 0.91 | 0.76 | 0.74 | 0.75 | 0.91 | 0.76 | 0.74 | 0.75 | 0.90 | 0.75 | 0.74 |
| $C\mathbf{H}_2O$ | 0.77 | 0.97 | 0.81 | 0.70 | 0.77 | 0.97 | 0.80 | 0.70 | 0.77 | 0.97 | 0.80 | 0.69 |
| $C\mathbf{H}_3F$ | 0.85 | 0.97 | 0.81 | 0.61 | 0.85 | 0.97 | 0.81 | 0.61 | 0.85 | 0.96 | 0.80 | 0.60 |
| $C_2\mathbf{H}_4$ | 0.79 | 0.96 | 0.80 | 0.65 | 0.79 | 0.96 | 0.80 | 0.65 | 0.79 | 0.96 | 0.80 | 0.64 |
| $\mathbf{H}_2O\cdots\mathbf{H}F$ | – | 0.90 | 0.74 | 0.63 | – | – | – | 0.63 | – | – | – | 0.63 |
| $\mathbf{H}_2O\cdots\mathbf{H}Cl$ | – | – | 0.74 | – | 0.63 | – | 0.74 | – | – | 0.92 | 0.74 | – |
| $\mathbf{H}_2O\cdots\mathbf{H}_2O$ | – | – | – | 0.62 | – | 0.90 | 0.75 | 0.61 | 0.60 | 0.90 | 0.75 | 0.61 |

Table S9: *f*-rank scores computed with NEO-DFT using spherical protonic basis sets. Bold fonts denote protons, which were treated as quantum particles. Omitted values correspond to computations, which did not converge or converged to wrong minima.

| Molecule | PB4-D | | | PB4-F1 | | | PB4-F2 | | |
|---|---|---|---|---|---|---|---|---|---|
| | HOi | 1s | core | HOi | 1s | core | HOi | 1s | core |
| F**H**F$^-$ | 0.95 | 0.71 | 0.75 | 0.93 | 0.71 | 0.76 | 0.93 | 0.71 | 0.76 |
| HO**H**$\cdots$FH | 0.90 | 0.72 | 0.73 | 0.91 | 0.72 | 0.74 | 0.91 | 0.72 | 0.74 |
| HO**H**$\cdots$ClH | 0.97 | 0.73 | 0.75 | 0.98 | 0.73 | 0.75 | 0.98 | 0.73 | 0.75 |
| $H_2O\cdots$**H**OH | 0.91 | 0.75 | 0.74 | 0.92 | 0.76 | 0.75 | 0.92 | 0.76 | 0.75 |
| $CH_3OH\cdots$**H**OH | 0.91 | 0.75 | 0.74 | 0.92 | 0.76 | 0.75 | 0.92 | 0.76 | 0.75 |
| H**H**NO | 0.96 | 0.78 | 0.76 | 0.96 | 0.79 | 0.77 | 0.96 | 0.79 | 0.77 |
| HO**H** | 0.90 | 0.76 | 0.75 | 0.91 | 0.77 | 0.75 | 0.91 | 0.77 | 0.75 |
| HS**H** | 0.98 | 0.77 | 0.76 | 0.98 | 0.78 | 0.77 | 0.98 | 0.78 | 0.77 |
| **H**CN | 0.94 | 0.78 | 0.76 | 0.95 | 0.79 | 0.77 | 0.95 | 0.79 | 0.77 |
| **H**FCO | 0.96 | 0.80 | 0.77 | 0.97 | 0.81 | 0.78 | 0.97 | 0.81 | 0.78 |
| **H**NO | 0.97 | 0.79 | 0.76 | 0.97 | 0.80 | 0.77 | 0.97 | 0.80 | 0.77 |
| **H**OCl | 0.91 | 0.76 | 0.75 | 0.92 | 0.77 | 0.76 | 0.92 | 0.77 | 0.76 |
| **H**OF | 0.91 | 0.76 | 0.75 | 0.92 | 0.77 | 0.76 | 0.92 | 0.77 | 0.76 |
| **H**ONO | 0.91 | 0.76 | 0.75 | 0.92 | 0.77 | 0.76 | 0.92 | 0.77 | 0.76 |
| $C\mathbf{H}_2O$ | 0.97 | – | – | 0.98 | 0.82 | 0.72 | 0.98 | 0.82 | 0.71 |
| $C\mathbf{H}_3F$ | 0.97 | 0.81 | 0.62 | 0.97 | 0.82 | 0.63 | 0.97 | 0.82 | 0.63 |
| $C_2\mathbf{H}_4$ | 0.97 | 0.81 | 0.66 | 0.97 | 0.82 | 0.67 | 0.97 | 0.82 | 0.67 |
| $\mathbf{H}_2O\cdots\mathbf{H}F$ | – | – | 0.64 | – | 0.75 | 0.65 | – | – | 0.64 |
| $\mathbf{H}_2O\cdots\mathbf{H}Cl$ | – | – | – | 0.93 | 0.75 | 0.65 | 0.93 | 0.75 | 0.65 |
| $\mathbf{H}_2O\cdots\mathbf{H}_2O$ | 0.90 | – | 0.62 | – | – | 0.63 | – | – | 0.63 |

Table S10: $f$-rank scores computed with NEO-DFT using spherical protonic basis sets. Bold fonts denote protons, which were treated as quantum particles. Omitted values correspond to computations, which did not converge or converged to wrong minima.

| Molecule | PB5-D | | | PB5-F | | | PB5-G | | |
|---|---|---|---|---|---|---|---|---|---|
| | HOi | 1s | core | HOi | 1s | core | HOi | 1s | core |
| F**H**F$^-$ | 0.94 | 0.71 | 0.76 | 0.93 | 0.71 | 0.76 | 0.94 | 0.71 | 0.76 |
| HO**H**$\cdots$FH | 0.90 | 0.72 | 0.74 | 0.91 | 0.73 | 0.74 | 0.91 | 0.73 | 0.74 |
| HO**H**$\cdots$ClH | 0.97 | 0.73 | 0.75 | 0.98 | 0.74 | 0.76 | 0.98 | 0.74 | 0.76 |
| $H_2O\cdots$**H**OH | 0.92 | 0.76 | 0.75 | 0.92 | 0.76 | 0.76 | 0.92 | 0.76 | 0.76 |
| $CH_3OH\cdots$**H**OH | 0.92 | 0.76 | 0.75 | 0.92 | 0.76 | 0.75 | 0.92 | 0.76 | 0.75 |
| H**H**NO | 0.96 | 0.79 | 0.77 | 0.96 | 0.79 | 0.77 | 0.96 | 0.79 | 0.77 |
| HO**H** | 0.90 | 0.77 | 0.75 | 0.91 | 0.77 | 0.76 | 0.91 | 0.77 | 0.76 |
| HS**H** | 0.98 | 0.78 | 0.77 | 0.98 | 0.78 | 0.77 | 0.98 | 0.78 | 0.77 |
| **H**CN | 0.95 | 0.79 | 0.77 | 0.95 | 0.79 | 0.77 | 0.95 | 0.79 | 0.77 |
| **H**FCO | 0.97 | 0.81 | 0.78 | 0.97 | 0.81 | 0.78 | 0.97 | 0.81 | 0.78 |
| **H**NO | 0.97 | 0.80 | 0.77 | 0.97 | 0.80 | 0.78 | 0.97 | 0.80 | 0.77 |
| **H**OCl | 0.91 | 0.77 | 0.76 | 0.92 | 0.77 | 0.76 | 0.91 | 0.77 | 0.76 |
| **H**OF | 0.92 | 0.77 | 0.76 | 0.92 | 0.78 | 0.76 | 0.92 | 0.77 | 0.76 |
| **H**ONO | 0.91 | 0.77 | 0.76 | 0.92 | 0.77 | 0.76 | 0.92 | 0.77 | 0.76 |
| C$\mathbf{H}_2$O | 0.97 | 0.82 | 0.71 | 0.98 | 0.82 | 0.71 | 0.98 | 0.82 | 0.71 |
| C$\mathbf{H}_3$F | 0.97 | 0.82 | 0.62 | 0.97 | 0.82 | 0.62 | 0.97 | 0.82 | 0.62 |
| $C_2\mathbf{H}_4$ | 0.97 | 0.82 | 0.66 | 0.97 | 0.82 | 0.67 | 0.97 | 0.82 | 0.67 |
| $\mathbf{H}_2O\cdots$**H**F | 0.90 | – | – | 0.91 | 0.75 | 0.65 | – | – | – |
| $\mathbf{H}_2O\cdots$**H**Cl | – | – | – | – | – | – | – | – | – |
| $\mathbf{H}_2O\cdots\mathbf{H}_2O$ | – | 0.77 | 0.63 | 0.91 | 0.77 | – | 0.91 | 0.77 | – |

# S4 Exponents from HOi

Table S11: Values of exponents $\zeta$ computed within the HOi approach from HF and DFT partial Hessians. Bold fonts denote protons, which were treated as quantum particles. See the main text for more details. Values are given in $\text{bohr}^{-2}$ units.

| Molecule | HF | DFT |
|---|---|---|
| F**H**F$^-$ | 6.00 | 5.87 |
| HO**H**$\cdots$FH | 17.07 | 13.92 |
| HO**H**$\cdots$ClH | 12.50 | 10.23 |
| $H_2O\cdots$**H**OH | 16.68 | 14.29 |
| $CH_3OH\cdots$**H**OH | 16.61 | 14.26 |
| H**H**NO | 14.23 | 12.30 |
| HO**H** | 16.94 | 15.24 |
| HS**H** | 11.79 | 10.83 |
| **H**CN | 14.13 | 13.27 |
| **H**FCO | 13.19 | 12.08 |
| **H**NO | 13.37 | 10.77 |
| **H**OCl | 16.72 | 14.81 |
| **H**OF | 16.62 | 14.63 |
| **H**ONO | 16.73 | 14.76 |

# S5 Numbers of SCF iterations

Table S12: Numbers of SCF iterations in the simultaneous NEO-HF convergence algorithm. Cartesian basis sets were employed. Bold fonts denote protons, which were treated as quantum particles. Omitted values correspond to computations, which did not converge or converged to wrong minima.

| Molecule | PB4-D | | | | PB4-F1 | | | | PB4-F2 | | | |
|---|---|---|---|---|---|---|---|---|---|---|---|---|
| | HOa | HOi | 1s | core | HOa | HOi | 1s | core | HOa | HOi | 1s | core |
| F**H**F$^-$ | 148 | 120 | 76 | 75 | 115 | 106 | 80 | 74 | 110 | 96 | 79 | 62 |
| HO**H**$\cdots$FH | 128 | 107 | 101 | 77 | 134 | 124 | 99 | 80 | 132 | 97 | 106 | 89 |
| HO**H**$\cdots$ClH | 150 | 98 | 82 | 90 | 175 | 99 | 115 | 102 | 157 | 95 | 103 | 117 |
| $H_2O\cdots$**H**OH | 135 | 119 | 101 | 101 | 150 | 110 | 128 | 95 | 177 | 120 | 107 | 104 |
| $CH_3OH\cdots$**H**OH | 150 | 129 | 206 | 119 | 189 | 129 | 123 | 121 | 167 | 139 | 132 | 186 |
| H**H**NO | 81 | 74 | 83 | 66 | 91 | 79 | 84 | 72 | 99 | 85 | 84 | 66 |
| HO**H** | 107 | 72 | 67 | 74 | 101 | 101 | 76 | 107 | 98 | 102 | 96 | 90 |
| HS**H** | 99 | 100 | 106 | 96 | 141 | 129 | 103 | 94 | 147 | 158 | 99 | 105 |
| **H**CN | 87 | 71 | 63 | 53 | 76 | 66 | 62 | 50 | 95 | 71 | 68 | 53 |
| **H**FCO | 115 | 131 | 120 | 160 | 148 | 112 | 114 | 118 | 138 | 123 | 120 | 97 |
| **H**NO | 99 | 117 | 100 | 89 | 126 | 94 | 136 | 84 | 147 | 104 | 114 | 91 |
| **H**OCl | 146 | 112 | 157 | 106 | 140 | 133 | 132 | 107 | 154 | 144 | 112 | 118 |
| **H**OF | 110 | 126 | 91 | 96 | 120 | 111 | 110 | 102 | 118 | 119 | 121 | 112 |
| **H**ONO | 149 | 109 | 192 | 114 | 124 | 121 | 107 | 111 | 147 | 114 | 122 | 108 |
| C$\mathbf{H}_2$O | 146 | 104 | 90 | 103 | 109 | 104 | 110 | 114 | 97 | 126 | 99 | 137 |
| C$\mathbf{H}_3$F | 103 | 96 | 61 | 107 | 103 | 96 | 71 | 113 | 121 | 101 | 71 | 130 |
| $C_2\mathbf{H}_4$ | 95 | 88 | 82 | 96 | 141 | 118 | 109 | 96 | 137 | 106 | 106 | 108 |
| $\mathbf{H}_2O\cdots$**H**F | 248 | 225 | 278 | 166 | 174 | 159 | 168 | 163 | 190 | 176 | 158 | 168 |
| $\mathbf{H}_2O\cdots$**H**Cl | 176 | – | – | 155 | 199 | 173 | 169 | 146 | 165 | 170 | 203 | 156 |
| $\mathbf{H}_2O\cdots\mathbf{H}_2O$ | 200 | 147 | 198 | 172 | – | – | – | 172 | – | – | – | 169 |

Table S13: Numbers of SCF iterations in the simultaneous NEO-HF convergence algorithm. Spherical basis sets were employed. Bold fonts denote protons, which were treated as quantum particles. Omitted values correspond to computations, which did not converge or converged to wrong minima.

| Molecule | PB4-D | | | PB4-F1 | | | PB4-F2 | | |
|---|---|---|---|---|---|---|---|---|---|
| | HOi | 1s | core | HOi | 1s | core | HOi | 1s | core |
| F**H**F$^-$ | 47 | 45 | 69 | 83 | 89 | 42 | 54 | 58 | 42 |
| HO**H**$\cdots$FH | 168 | 102 | 84 | 94 | 101 | 93 | 96 | 101 | 83 |
| HO**H**$\cdots$ClH | 86 | 107 | 78 | 91 | 152 | 106 | 93 | 93 | 83 |
| $H_2O\cdots$**H**OH | 102 | 83 | 83 | 112 | 92 | 90 | 93 | 108 | 93 |
| $CH_3OH\cdots$**H**OH | 140 | 138 | 122 | 141 | 132 | 133 | 149 | 122 | 130 |
| H**H**NO | 81 | 80 | 63 | 83 | 89 | 58 | 74 | 91 | 66 |
| HO**H** | 103 | 101 | 71 | 112 | 97 | 60 | 97 | 97 | 58 |
| HS**H** | 130 | 88 | 76 | 100 | 106 | 74 | 113 | 120 | 74 |
| **H**CN | 61 | 60 | 53 | 62 | 62 | 49 | 68 | 68 | 49 |
| **H**FCO | 109 | 114 | 76 | 116 | 110 | 88 | 107 | 105 | 80 |
| **H**NO | 92 | 105 | 82 | 88 | 101 | 88 | 126 | 104 | 80 |
| **H**OCl | 103 | 94 | 91 | 114 | 93 | 83 | 105 | 100 | 94 |
| **H**OF | 98 | 84 | 82 | 106 | 89 | 82 | 115 | 107 | 79 |
| **H**ONO | 110 | 107 | 111 | 115 | 120 | 111 | 120 | 107 | 125 |
| C$\mathbf{H}_2$O | 93 | 80 | 111 | 90 | 109 | 100 | 132 | 115 | 106 |
| C$\mathbf{H}_3$F | 87 | 79 | 99 | 82 | 83 | 104 | 83 | 82 | 130 |
| $C_2\mathbf{H}_4$ | 130 | 96 | 80 | 91 | 90 | 109 | 87 | 111 | 89 |
| $\mathbf{H}_2O\cdots$**H**F | – | – | 155 | 152 | 159 | 148 | 157 | 137 | 165 |
| $\mathbf{H}_2O\cdots$**H**Cl | – | – | 145 | – | – | 159 | – | – | 148 |
| $\mathbf{H}_2O\cdots\mathbf{H}_2O$ | 119 | 119 | 174 | 158 | 156 | 166 | 154 | 185 | 184 |

Table S14: Numbers of SCF iterations in the simultaneous NEO-HF convergence algorithm. Spherical basis sets were employed. Bold fonts denote protons, which were treated as quantum particles. Omitted values correspond to computations, which did not converge or converged to wrong minima.

| Molecule | PB5-D | | | PB5-F | | | PB5-G | | |
|---|---|---|---|---|---|---|---|---|---|
| | HOi | 1s | core | HOi | 1s | core | HOi | 1s | core |
| F**H**F$^-$ | 94 | 92 | 50 | 77 | 82 | 67 | 60 | 68 | 48 |
| HO**H**$\cdots$FH | 135 | 113 | 158 | 110 | 122 | 112 | 108 | 100 | 125 |
| HO**H**$\cdots$ClH | 90 | 125 | 111 | 97 | 111 | 127 | 90 | 98 | 106 |
| $H_2O\cdots$**H**OH | 119 | 111 | 88 | 114 | 101 | 104 | 104 | 108 | 114 |
| $CH_3OH\cdots$**H**OH | 152 | 132 | 137 | 146 | 145 | 130 | 168 | 137 | 119 |
| H**H**NO | 87 | 92 | 77 | 86 | 92 | 69 | 81 | 75 | 74 |
| HO**H** | 92 | 96 | 79 | 111 | 90 | 63 | 92 | 96 | 68 |
| HS**H** | 113 | 100 | 108 | 144 | 109 | 118 | 155 | 114 | 95 |
| **H**CN | 84 | 79 | 57 | 79 | 78 | 63 | 73 | 64 | 56 |
| **H**FCO | 116 | 109 | 133 | 113 | 129 | 149 | 118 | 121 | 114 |
| **H**NO | 108 | 114 | 100 | 102 | 110 | 99 | 160 | 123 | 84 |
| **H**OCl | 121 | 124 | 102 | – | – | 117 | – | – | 103 |
| **H**OF | 114 | 98 | 89 | 101 | 107 | 100 | 114 | 101 | 112 |
| **H**ONO | 119 | 130 | 94 | 118 | 134 | 134 | 117 | – | 138 |
| C**H**$_2$O | 111 | 105 | 135 | 105 | 107 | 107 | 125 | 122 | 141 |
| C**H**$_3$F | 106 | 105 | 120 | 100 | 95 | 106 | 112 | 89 | 116 |
| C$_2$**H**$_4$ | 95 | 91 | 94 | 119 | 104 | 99 | 145 | 106 | 132 |
| **H**$_2$O$\cdots$**H**F | 143 | 155 | 159 | 171 | 149 | 154 | 149 | 156 | 183 |
| **H**$_2$O$\cdots$**H**Cl | 157 | 153 | 155 | 160 | 170 | 154 | 182 | 177 | 160 |
| **H**$_2$O$\cdots$**H**$_2$O | – | 229 | 169 | 296 | – | 184 | – | – | 192 |

Table S15: Numbers of SCF iterations in the simultaneous NEO-DFT convergence algorithm. Cartesian basis sets were employed. Bold fonts denote protons, which were treated as quantum particles. Omitted values correspond to computations, which did not converge or converged to wrong minima.

| Molecule | PB4-D | | | | PB4-F1 | | | | PB4-F2 | | | |
|---|---|---|---|---|---|---|---|---|---|---|---|---|
| | HOa | HOi | 1s | core | HOa | HOi | 1s | core | HOa | HOi | 1s | core |
| F**H**$F^-$ | 59 | 119 | 153 | 131 | 87 | 65 | 147 | 66 | 178 | 65 | 199 | 78 |
| HO**H**···FH | 187 | 114 | 123 | 91 | 154 | 220 | 110 | 133 | 129 | 157 | 141 | 196 |
| HO**H**···ClH | 175 | 173 | 135 | 146 | 206 | 290 | 193 | 151 | 256 | 172 | 231 | 176 |
| $H_2O$···**H**OH | 191 | 110 | 129 | 241 | 140 | 131 | 162 | 222 | 166 | 150 | 211 | 167 |
| $CH_3OH$···**H**OH | 160 | 145 | 125 | 161 | 286 | 152 | 203 | 179 | 251 | 201 | 230 | 198 |
| H**H**NO | 121 | 84 | 98 | 148 | 121 | 103 | 190 | 166 | 128 | 105 | 154 | 153 |
| HO**H** | 63 | 93 | 82 | 92 | 72 | 97 | 208 | 121 | 89 | 100 | 88 | 133 |
| HS**H** | 113 | 93 | 160 | 172 | 121 | 101 | 188 | 144 | 93 | 120 | 122 | 137 |
| **H**CN | 70 | 77 | 85 | 78 | 95 | 78 | 67 | 93 | 194 | 84 | 94 | 78 |
| **H**FCO | 158 | 110 | 121 | 108 | 207 | 98 | 125 | 119 | 166 | 116 | 152 | 129 |
| **H**NO | 105 | 105 | 123 | 114 | 177 | 102 | 110 | 112 | 128 | 106 | 134 | 184 |
| **H**OCl | 151 | 136 | 118 | 158 | 253 | 189 | 148 | 173 | 125 | 199 | 118 | 196 |
| **H**OF | 115 | 129 | 99 | 124 | 104 | 137 | 127 | 95 | 197 | 139 | 109 | 171 |
| **H**ONO | 170 | 112 | 160 | 185 | 160 | 158 | 235 | 183 | – | 154 | 143 | 260 |
| C$\mathbf{H}_2$O | 104 | 139 | 135 | 128 | 166 | 120 | 126 | 143 | 135 | 120 | 148 | 111 |
| C$\mathbf{H}_3$F | 122 | 143 | 111 | 127 | 113 | 103 | 105 | 126 | 204 | 80 | 134 | 207 |
| $C_2\mathbf{H}_4$ | 129 | 103 | 98 | 105 | 148 | 116 | 136 | 229 | 125 | 121 | 129 | 155 |
| $\mathbf{H}_2$O···**H**F | – | 156 | 140 | 215 | – | – | – | 265 | – | – | – | 225 |
| $\mathbf{H}_2$O···**H**Cl | – | – | 296 | – | 269 | – | 280 | – | – | 273 | 285 | – |
| $\mathbf{H}_2$O···$\mathbf{H}_2$O | – | – | – | 284 | – | 272 | 180 | 274 | 214 | 228 | 274 | 252 |

Table S16: Numbers of SCF iterations in the simultaneous NEO-DFT convergence algorithm. Spherical basis sets were employed. Bold fonts denote protons, which were treated as quantum particles. Omitted values correspond to computations, which did not converge or converged to wrong minima.

| Molecule | PB4-D | | | PB4-F1 | | | PB4-F2 | | |
|---|---|---|---|---|---|---|---|---|---|
| | HOi | 1s | core | HOi | 1s | core | HOi | 1s | core |
| F**H**F$^-$ | 74 | 62 | 38 | 78 | 39 | 53 | 40 | 39 | 54 |
| HO**H**$\cdots$FH | 96 | 135 | 158 | 104 | 127 | 93 | 109 | 130 | 95 |
| HO**H**$\cdots$ClH | 124 | 174 | 204 | 82 | 140 | 100 | 97 | 113 | 130 |
| $H_2O\cdots$**H**OH | 124 | 185 | 127 | 136 | 151 | 113 | 159 | 98 | 132 |
| $CH_3OH\cdots$**H**OH | 188 | 228 | 176 | 161 | 239 | 165 | 148 | 167 | 115 |
| H**H**NO | 89 | 91 | 99 | 98 | 93 | 79 | 81 | 93 | 76 |
| HO**H** | 76 | 69 | 106 | 111 | 87 | 68 | 85 | 94 | 79 |
| HS**H** | 128 | 119 | 105 | 146 | 117 | 123 | 100 | 172 | 94 |
| **H**CN | 69 | 62 | 58 | 61 | 71 | 73 | 58 | 68 | 65 |
| **H**FCO | 137 | 126 | 98 | 98 | 92 | 80 | 120 | 115 | 80 |
| **H**NO | 84 | 140 | 136 | 90 | 75 | 127 | 93 | 100 | 118 |
| **H**OCl | 124 | 98 | 219 | 182 | 115 | 161 | 117 | 107 | 146 |
| **H**OF | 93 | 96 | 155 | 96 | 90 | 128 | 128 | 118 | 108 |
| **H**ONO | 112 | 195 | 207 | 119 | 132 | 96 | 123 | 144 | 103 |
| C$\mathbf{H}_2$O | 98 | – | – | 75 | 109 | 105 | 66 | 106 | 112 |
| C$\mathbf{H}_3$F | 83 | 100 | 114 | 72 | 93 | 94 | 80 | 84 | 85 |
| $C_2\mathbf{H}_4$ | 82 | 137 | 214 | 130 | 82 | 135 | 108 | 85 | 121 |
| $\mathbf{H}_2O\cdots$**H**F | – | – | 286 | – | 286 | 133 | – | – | 216 |
| $\mathbf{H}_2O\cdots$**H**Cl | – | – | – | 212 | 199 | 194 | 223 | 226 | 286 |
| $\mathbf{H}_2O\cdots\mathbf{H}_2O$ | 286 | – | 265 | – | – | 233 | – | – | 182 |

Table S17: Numbers of SCF iterations in the simultaneous NEO-DFT convergence algorithm. Spherical basis sets were employed. Bold fonts denote protons, which were treated as quantum particles. Omitted values correspond to computations, which did not converge or converged to wrong minima.

| Molecule | PB5-D | | | PB5-F | | | PB5-G | | |
|---|---|---|---|---|---|---|---|---|---|
| | HOi | 1s | core | HOi | 1s | core | HOi | 1s | core |
| F**H**F$^-$ | 73 | 73 | 79 | 66 | 70 | 73 | 60 | 71 | 71 |
| HO**H**$\cdots$FH | 164 | 175 | 167 | 130 | 145 | 177 | 168 | 113 | 177 |
| HO**H**$\cdots$ClH | 183 | 231 | – | 173 | 202 | 215 | 147 | 247 | 180 |
| $H_2O\cdots$**H**OH | 159 | 202 | 178 | 149 | 199 | 138 | 178 | 182 | 182 |
| $CH_3OH\cdots$**H**OH | 206 | 211 | 202 | 176 | 264 | 183 | 170 | 243 | 198 |
| H**H**NO | 103 | 77 | 136 | 96 | 115 | 121 | 81 | 90 | 103 |
| HO**H** | 102 | 109 | 90 | 109 | 125 | 92 | 87 | 75 | 93 |
| HS**H** | 111 | 239 | 210 | 121 | 132 | 192 | 142 | 227 | 213 |
| **H**CN | 77 | 73 | 106 | 69 | 103 | 86 | 80 | 103 | 100 |
| **H**FCO | 188 | 148 | 123 | 119 | 144 | 111 | 121 | 159 | 136 |
| **H**NO | 102 | 185 | 112 | 119 | 143 | 223 | 105 | 133 | 188 |
| **H**OCl | 206 | 103 | 165 | 192 | 154 | 137 | 191 | 162 | 218 |
| **H**OF | 138 | 110 | 131 | 131 | 125 | 162 | 120 | 163 | 151 |
| **H**ONO | 170 | 177 | 177 | 166 | 205 | 171 | 157 | 196 | 210 |
| C**H**$_2$O | 173 | 124 | 135 | 144 | 144 | 139 | 117 | 138 | 144 |
| C**H**$_3$F | 93 | 132 | 134 | 116 | 116 | 218 | 112 | 119 | 156 |
| $C_2$**H**$_4$ | 139 | 113 | 200 | 140 | 140 | 175 | 139 | 147 | 161 |
| **H**$_2$O$\cdots$**H**F | 188 | – | – | 233 | 233 | 280 | – | – | – |
| **H**$_2$O$\cdots$**H**Cl | – | – | – | – | – | – | – | – | – |
| **H**$_2$O$\cdots$**H**$_2$O | – | 209 | 288 | 274 | 274 | – | 221 | 297 | – |

# References


[1] J. Zinn-Justin. *Quantum field theory and critical phenomena.* Oxford University Press, 4 ed., 2021.

[2] S. P. Webb, T. Iordanov, S. Hammes-Schiffer. Multiconfigurational nuclear-electronic orbital approach: Incorporation of nuclear quantum effects in electronic structure calculations. *J. Chem. Phys.*, **117** (2002) 4106–4118.

[3] M. V. Pak, A. Chakraborty, S. Hammes-Schiffer. Density Functional Theory Treatment of Electron Correlation in the Nuclear–Electronic Orbital Approach. *J. Phys. Chem. A*, **111** (2007) 4522–4526.

[4] A. Chakraborty, M. V. Pak, S. Hammes-Schiffer. Development of Electron–Proton Density Functionals for Multicomponent Density Functional Theory. *Phys. Rev. Lett.*, **101** (2008) 153001.

[5] A. Chakraborty, M. V. Pak, S. Hammes-Schiffer. Properties of the exact universal functional in multicomponent density functional theory. *J. Chem. Phys.*, **131** (2009) 124115.

[6] A. Sirjoosingh, M. V. Pak, S. Hammes-Schiffer. Derivation of an Electron–Proton Correlation Functional for Multicomponent Density Functional Theory within the Nuclear–Electronic Orbital Approach. *J. Chem. Theory Comput.*, **7** (2011) 2689–2693.

[7] A. Sirjoosingh, M. V. Pak, S. Hammes-Schiffer. Multicomponent density functional theory study of the interplay between electron–electron and electron–proton correlation. *J. Chem. Phys.*, **136** (2012) 174114.

[8] J. P. Unsleber, T. Dresselhaus, K. Klahr, D. Schnieders, M. Böckers, D. Barton, J. Neugebauer. Serenity: A subsystem quantum chemistry program. *J. Comput. Chem.*, **39** (2018) 788–798.

[9] N. Niemeyer, P. Eschenbach, M. Bensberg, J. Tölle, L. Hellmann, L. Lampe, A. Massolle, A. Rikus, D. Schnieders, J. P. Unsleber, J. Neugebauer. The subsystem quantum chemistry program SERENITY. *WIREs Comput. Mol. Sci.*, **13** (2023) e1647.

[10] D. Artiukhin, D. Barton, M. Bensberg, M. Böckers, T. Dresselhaus, P. Eschenbach, L. Fischer, N. Göllmann, L. Hellmann, L. Lampe, A. Massolle, N. Niemeyer, L. Paetow, N. Ramez, A. Rikus, D. Schnieders, J. Tölle, J. P. Unsleber, K. Wegner, T. Wiegmann, J. Neugebauer. qcserenity/serenity: Release 1.6.3, April 2025.

[11] Yihan Shao, Zhengting Gan, Evgeny Epifanovsky, Andrew T. B. Gilbert, Michael Wormit, Joerg Kussmann, Adrian W. Lange, Andrew Behn, Jia Deng, Xintian Feng, Debashree Ghosh, Matthew Goldey, Paul R. Horn, Leif D. Jacobson, Ilya Kaliman, Rustam Z. Khaliullin, Tomasz Kuś, Arie Landau, Jie Liu, Emil I. Proynov, Young Min Rhee, Ryan M. Richard, Mary A. Rohrdanz, Ryan P. Steele, Eric J. Sundstrom, H. Lee Woodcock III, Paul M. Zimmerman, Dmitry Zuev, Ben Albrecht, Ethan Alguire, Brian Austin, Gregory J. O. Beran, Yves A. Bernard, Eric Berquist, Kai Brandhorst, Ksenia B. Bravaya, Shawn T. Brown, David Casanova, Chun-Min Chang, Yunqing Chen, Siu Hung Chien, Kristina D. Closser, Deborah L. Crittenden, Michael Diedenhofen, Robert A. DiStasio Jr., Hainam Do, Anthony D. Dutoi, Richard G. Edgar, Shervin Fatehi, Laszlo Fusti-Molnar, An Ghysels, Anna Golubeva-Zadorozhnaya, Joseph Gomes, Magnus W. D. Hanson-Heine, Philipp H. P. Harbach, Andreas W. Hauser, Edward G. Hohenstein, Zachary C. Holden, Thomas-C. Jagau, Hyunjun Ji, Benjamin Kaduk, Kirill Khistyaev, Jaehoon Kim, Jihan Kim, Rollin A. King, Phil Klunzinger, Dmytro Kosenkov, Tim Kowalczyk, Caroline M. Krauter, Ka Un Lao, Adèle D. Laurent, Keith V. Lawler, Sergey V.

Levchenko, Ching Yeh Lin, Fenglai Liu, Ester Livshits, Rohini C. Lochan, Arne Luenser, Prashant Manohar, Samuel F. Manzer, Shan-Ping Mao, Narbe Mardirossian, Aleksandr V. Marenich, Simon A. Maurer, Nicholas J. Mayhall, Eric Neuscamman, C. Melania Oana, Roberto Olivares-Amaya, Darragh P. O'Neill, John A. Parkhill, Trilisa M. Perrine, Roberto Peverati, Alexander Prociuk, Daniel R. Rehn, Edina Rosta, Nicholas J. Russ, Shaama M. Sharada, Sandeep Sharma, David W. Small, Alex Sodt, Tamar Stein, David Stück, Yu-Chuan Su, Alex J. W. Thom, Takashi Tsuchimochi, Vlad Vanovschi, Leslie Vogt, Oleg Vydrov, Tao Wang, Mark A. Watson, Jan Wenzel, Alec White, Christopher F. Williams, Jun Yang, Sina Yeganeh, Shane R. Yost, Zhi-Qiang You, Igor Ying Zhang, Xing Zhang, Yan Zhao, Bernard R. Brooks, Garnet K.-L. Chan, Daniel M. Chipman, Christopher J. Cramer, William A. Goddard, Mark S. Gordon, Warren J. Hehre, Andreas Klamt, Henry F. Schaefer III, Michael W. Schmidt, C. David Sherrill, Donald G. Truhlar, Arieh Warshel, Xin Xu, Alán Aspuru-Guzik, Roi Baer, Alexis T. Bell, Nicholas A. Besley, Jeng-Da Chai, Andreas Dreuw, Barry D. Dunietz, Thomas R. Furlani, Steven R. Gwaltney, Chao-Ping Hsu, Yousung Jung, Jing Kong, Daniel S. Lambrecht, Wanzhen Liang, Christian Ochsenfeld, Vitaly A. Rassolov, Lyudmila V. Slipchenko, Joseph E. Subotnik, Troy Van Voorhis, John M. Herbert, Anna I. Krylov, Peter M. W. Gill, Martin Head-Gordon. Advances in molecular quantum chemistry contained in the q-chem 4 program package. *Molecular Physics*, **113**(2) (2015) 184–215.

[12] Q. Yu, F. Pavošević, S. Hammes-Schiffer. Development of nuclear basis sets for multicomponent quantum chemistry methods. *J. Chem. Phys.*, **152** (2020) 244123.
